# Supplementary material for: Wi-Fi Assist: Enhancing Vehicular Wi-Fi Connectivity with an Infrastructure-driven Approach
Source: arXiv:2207.04547 source file (2022-07-10)
Supplement: Supplementary file 1 [file appendix.tex]

%APPENDICES are optional
%\balancecolumns
\appendix
%Appendix A
